# Supplementary material for: Tree-aggregated compositional regression under measurement error
Source: arXiv:2605.15469 source file (2026-11-16)
Supplement: Supplementary file 1 [file supplement_numbers.tex]

% Supplement reference numbers for the main-only preprint.
\makeatletter
\@namedef{suppnumber@prop:penalty_boundary_supp}{S16}
\@namedef{suppnumber@rem:pointwise_reference_comparison}{S13}
\@namedef{suppnumber@sec:additional_application_appendix}{S12}
\@namedef{suppnumber@sec:additional_simulation_appendix}{S11}
\@namedef{suppnumber@sec:common_event}{S6}
\@namedef{suppnumber@sec:cv_appendix}{S13}
\@namedef{suppnumber@sec:error_amplification_proof}{S3}
\@namedef{suppnumber@sec:fixed_comparison}{S1.1}
\@namedef{suppnumber@sec:induced_norm}{S5}
\@namedef{suppnumber@sec:projection}{S4}
\@namedef{suppnumber@sec:replicate_supp}{S9}
\@namedef{suppnumber@sec:toy_example_appendix}{S10}
\@namedef{suppnumber@tab:application_groups_v1}{S4}
\@namedef{suppnumber@tab:benchmark_threshold}{S1}
\@namedef{suppnumber@tab:extra_comparators_main}{S2}
\@namedef{suppnumber@tab:extra_comparators_tau}{S3}
\@namedef{suppnumber@thm:deterministic_oracle_supp}{S22}
\newcommand{\suppref}[1]{\@nameuse{suppnumber@#1}}
\makeatother
